# Supplementary material for: Cross-layer Optimization for High Speed Adders: A Pareto Driven Machine Learning Approach
Source: arXiv:1807.07023 source file (2018-10-16)
Supplement: Supplementary file 1 [file appendix.tex]

\clearpage
\appendix

\begin{figure}[!h]
    \centering
	\subfloat[]{\includegraphics[width=0.35\textwidth]{space_AD}}\hspace{.1in}
	\subfloat[]{\includegraphics[width=0.35\textwidth]{space_AT}}\hspace{.1in}
	\subfloat[]{\includegraphics[width=0.35\textwidth]{space_PD}}\hspace{.1in}
	\subfloat[]{\includegraphics[width=0.35\textwidth]{space_PT}}
    \caption{Original Space vs.~3K points}
\end{figure}

\begin{figure}[!h]
     \centering
	 \subfloat[]{\includegraphics[width=0.35\textwidth]{AD}} \hspace{.1in}
	 \subfloat[]{\includegraphics[width=0.35\textwidth]{AT}} \hspace{.1in}
	 \subfloat[]{\includegraphics[width=0.35\textwidth]{PD}} \hspace{.1in}
	 \subfloat[]{\includegraphics[width=0.35\textwidth]{PT}}
     \caption{Real PF vs.~Predicted PF}
\end{figure}

\begin{figure}[!tbh]
    \centering
    \subfloat[]{\includegraphics[width=0.35\textwidth]{AT_zoom}} \hspace{.1in}  
	\subfloat[]{\includegraphics[width=0.35\textwidth]{PT_zoom}}
    \caption{
        (a) Area-TNS zoom in;
        (b) Power-TNS zoom in.
    }
\end{figure}
